# Supplementary material for: RobotCore: An Open Architecture for Hardware Acceleration in ROS 2
Source: arXiv:2205.03929 source file (2023-06-30)
Supplement: Supplementary file 1 [file appendix_figures.tex]

\begin{figure*}[p]
    \centering
    \begin{subfigure}[b]{0.45\textwidth}
        \centering
        \resizebox{0.6\textwidth}{!}{
            \begin{tikzpicture}   
                \pie[square, rotate=270, text=pin, color={lightgray!90, lightgray!70, lightgray!50, lightgray!30, lightgray!10}]  
                    {45.5/Medium, 27.3/High, 18.2/Very high, 9/Very low}  
               
            \end{tikzpicture}  
        }
        \caption{\footnotesize Distribution of respondents to the question: "What's your cybersecurity concern in PX4?". No respondents indicated "Low". \emph{Sample size 11 respondents.}}
        \label{fig:px4:1}
    \end{subfigure}
    ~
    \begin{subfigure}[b]{0.45\textwidth}
        \centering
        \resizebox{0.5\textwidth}{!}{
            \begin{tikzpicture}   
                \pie[rotate=270, text=inside, color={lightgray!90, lightgray!70, lightgray!50, lightgray!30, lightgray!10}]  
                    {72.7/Yes, 18.2/No, 9.1/Other}  
               
            \end{tikzpicture}  
        }
        \caption{\footnotesize Distribution of respondents to the question: "Does cyber security affect safety?". Other corresponds with user-provided answers. \emph{Sample size 11 respondents.}}
        \label{fig:px4:2}
    \end{subfigure}
    \\[5ex]
    \begin{subfigure}[b]{0.45\textwidth}
        \centering
        \resizebox{\textwidth}{!}{
            \begin{tikzpicture}   
                \pie[explode=0.2, polar, rotate=270, text=pin, color={lightgray!90, lightgray!70, lightgray!50, lightgray!30, lightgray!10}]  
                    {0/Yes, 80/No, 0/Only in industry, 20/Depends vendor or end-user}
            \end{tikzpicture}  
        }
        \caption{\footnotesize Distribution of respondents to the question: "Do you think security awareness is sufficient in robotics?". \emph{Sample size not provided by ERF's platform.}}
        \label{fig:erf:1}
    \end{subfigure}
    ~
    \begin{subfigure}[b]{0.45\textwidth}
        \centering
        \resizebox{0.8\textwidth}{!}{
            \begin{tikzpicture}   
                \pie[explode=0.2, polar, rotate=270, text=pin, color={lightgray!90, lightgray!70, lightgray!50, lightgray!30, lightgray!10}]  
                    {43/Vendor, 14/End-user, 43/System integrators, 0/Distributors, 0/Insurance providers}
            \end{tikzpicture}  
        }
        \caption{\footnotesize Distribution of respondents to the question: "Who is the actor to be responsible for cyberincidents?". \emph{Sample size not provided by ERF's platform.}}
        \label{fig:erf:2}
    \end{subfigure}
    \\[5ex]
    \begin{subfigure}[b]{0.3\textwidth}
        \resizebox{\textwidth}{!}{
            \begin{tikzpicture}
              \begin{axis}[
                xbar,
                xmin=0,
                y axis line style = { opacity = 0 },
                axis x line       = none,
                tickwidth         = 0pt,
                bar width         = 3em,
                enlarge y limits  = 0.2,
                enlarge x limits  = 0.02,
                symbolic y coords = {Public,Private,Total},
                nodes near coords,
                ytick             = data,                
              ]
              \addplot[black, fill=lightgray] coordinates { 
                (61,Public) 
                (15,Private) 
                (76,Total) 
             };
              %\legend{Percentage)}
              \end{axis}
            \end{tikzpicture}
        }
        \caption{\footnotesize Vulnerabilities affecting ABB robots registered in the {RVD} (Public), in other private databases (Private), as well as the overall amount (Total).}
        \label{fig:vulns:dist:abb}
    \end{subfigure}
    ~
    \begin{subfigure}[b]{0.3\textwidth}
        \resizebox{\textwidth}{!}{
            \begin{tikzpicture}
              \begin{axis}[
                xbar,
                xmin=0,
                y axis line style = { opacity = 0 },
                axis x line       = none,
                tickwidth         = 0pt,
                bar width         = 3em,
                enlarge y limits  = 0.2,
                enlarge x limits  = 0.02,
                symbolic y coords = {Public,Private,Total},
                nodes near coords,
                ytick             = data,                
              ]
              \addplot[black, fill=lightgray] coordinates { 
                (15,Public) 
                (125,Private) 
                (140,Total) 
             };
              %\legend{Percentage)}
              \end{axis}
            \end{tikzpicture}
        }
        \caption{\footnotesize Vulnerabilities affecting MiR robots registered in the {RVD} (Public), in other private databases (Private) as well as the overall amount (Total).}
        \label{fig:vulns:dist:mir}
    \end{subfigure}
    ~
    \begin{subfigure}[b]{0.3\textwidth}
        \resizebox{\textwidth}{!}{
            \begin{tikzpicture}
              \begin{axis}[
                xbar,
                xmin=0,
                y axis line style = { opacity = 0 },
                axis x line       = none,
                tickwidth         = 0pt,
                bar width         = 3em,
                enlarge y limits  = 0.2,
                enlarge x limits  = 0.02,
                symbolic y coords = {Public,Private,Total},
                nodes near coords,
                ytick             = data,                
              ]
              \addplot[black, fill=lightgray] coordinates { 
                (92,Public) 
                (367,Private) 
                (459,Total) 
             };
              %\legend{Percentage)}
              \end{axis}
            \end{tikzpicture}
        }
        \caption{\footnotesize Vulnerabilities affecting UR robots registered in the {RVD} (Public), in other private databases (Private) as well as the overall amount (Total).}
        \label{fig:vulns:dist:ur}
    \end{subfigure}

    \vspace{2em}
    \caption{\textbf{Surveying the PX4 robotics community (2020)}: Security survey launched within the PX4 Discourse community (\href{https://discuss.px4.io/t/cyber-security-in-px4-survey-and-input/17449}{announcement}).}
    \label{fig:survey}
\end{figure*}
